# Supplementary material for: Analytical model of atomic-force-microscopy force curves in viscoelastic materials exhibiting power law relaxation
Source: arXiv:1610.07180 source file (2016-10-23)
Supplement: Supplementary file 1 [file supmat_v3.pdf]

# Supplementary material: Analytical model of atomic-force-microscopy force curves in viscoelastic materials exhibiting power law relaxation

J. S. de Sousa[1], J. A. C. Santos[1,3], E. B. Barros[1], L. M. R. Alencar[2], W. T. Cruz[4], M. V. Ramos[4], J. Mendes Filho[1]
Departamento de Física, Universidade Federal do Ceará, Brazil
[2]Instituto Federal de Educação, Ciência e Tecnologia do Ceará, Brazil
[3]Universidade de Fortaleza, Brazil
[4]Departamento de Bioquímica e Biologia Molecular, Universidade Federal do Ceará, Brazil

October 6, 2016

## Contents

**1 Constitutive equation** **2**

**2 Quadratic indentation profile: force model for n=1 (SLS model)** **4**

**3 Error analysis** **6**

**4 Computational FEM validation** **9**

**5 Indentation profiles of the polyacrylamide force curves** **11**

**6 Indentation profiles of the PnBMA force curves** **12**

# 1 Constitutive equation

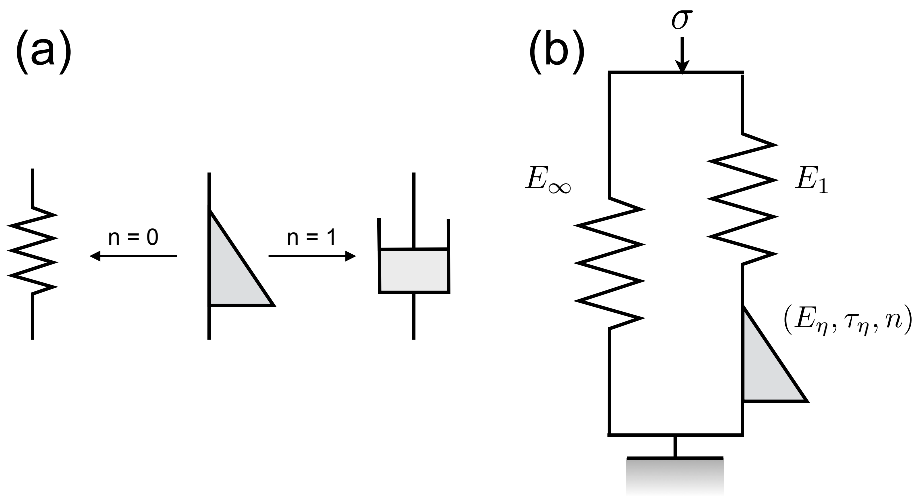


Figure 1: (a) Representation of a single fraction element. (b) The Fractional SLS model.

The constitutive stress-strain equation of a single fractional element, as shown in Figure 1(a), is given by:

$$\sigma(t) = \Lambda \frac{d^n \epsilon(t)}{dt^n}, \tag{1}$$

where $\sigma(t)$ is the stress, $\epsilon(t)$ is the strain, $d^n/dt^n$ is the fractional derivative operator ($0 \leq n \leq 1$), and $\Lambda$ is a material quasi-property (with SI units of Pa.s$^n$). One can write $\Lambda = E\tau^n$, such that a single fractional element is described by three parameters $(E, \tau, n)$. The fractional element interpolates between two responses: for $n = 0$ for a Hookean elastic spring that can be described only $E$ (since $n = 0$, $\tau$ becomes meaningless) , and $n = 1$ for a Newtonian dashpot. References regarding the mathematical properties of fractional elements are present in the manuscript. Figure 1(b) shows the fractional SLS model adopted in this work, whose stress-strain constitutive equation is given by:

$$\left(\frac{d^n}{dt^n} + \frac{1}{\tau_\epsilon^n}\right) \sigma(t) = G_0 \left(\frac{d^n}{dt^n} + \frac{1}{\tau_\sigma^n}\right) \epsilon(t), \tag{2}$$

where $E_0 = E_1 + E_\infty$, $\tau_\epsilon^n = (E_\eta/E_1)\tau_\eta^n$, and $\tau_\sigma^n = (E_0/E_\infty)\tau_\epsilon^n$ is the relaxation time for constant stress. The general fractional differentiation is based in the Caputo derivative defined as:

$${}_a^C D_t^n f(t) = \frac{1}{\Gamma(m-n)} \int_a^t (t-t')^{m-n-1} f^m(t') dt' \tag{3}$$

where $m-1 < n \leq m$, and $m$ is an integer. Assuming $f(t) = 0$ for $t \leq 0$, we obtain ${}_0^C D_t^n f(t) = d^n f(t)/dt^n$. The Laplace transform of the Caputo derivative is given by:

$$\mathcal{L}\left[\frac{d^n f(t)}{dt^n}\right] = s^n \tilde{f}(s) - \sum_{k=0}^{m-1} s^{n-k-1} f^{(k)}(0),\ m-1 < n \leq m. \tag{4}$$

Applying the above Laplace transform definition in the fractional constitutive equation (using $\sigma(0) = \epsilon(0) = 0$ as initial conditions), one obtains:

$$\tilde{\sigma}(s) = E_0 \left(\frac{s^n + \tau_\sigma^{-n}}{s^n + \tau_\epsilon^{-n}}\right) \tilde{\epsilon}(s) \tag{5}$$

Under the hypothesis of causal histories, the stress-strain relationship can be written as:

$$\sigma(t) = \int_0^t R(t-t') \frac{d}{dt'} \epsilon(t') dt', \tag{6}$$

whose Laplace transform is $\tilde{\sigma}(s) = s\tilde{R}(s)\tilde{\epsilon}(s)$. Thus, one obtains:

$$\tilde{R}(s) = E_0 \left[\frac{s + \tau_\sigma^{-1}}{s(s + \tau_\epsilon^{-1})}\right], \tag{7}$$

Finally, the relaxation function in time domain reads:

$$R(t) = E_\infty + E_1 E_{n,1}\left[-\left(\frac{t}{\tau}\right)^n\right] \tag{8}$$

where $E_{n,1}(z)$ is the generalized Mittag-Leffler function. For $n = 1$ one has $E_{1,1}(z) = \exp(z)$ which results in the shear relaxation function of the conventional SLS model. The elasticity modulus relaxes from the instantaneous $R(0) = E_0$ to the relaxed modulus $R(t \to \infty) = E_\infty$, where the amplitude of relaxation is $E_1 = E_0 - E_\infty$. Alternatively, one can write the relaxation function as:

$$R(t) = E_0 \left[(1-\alpha) + \alpha E_{n,1}\left[-\left(\frac{t}{\tau}\right)^n\right]\right] \tag{9}$$

where $\alpha$ is defined such that $E_1 = \alpha E_0$ and $E_\infty = (1-\alpha)E_0$.

## 2 Quadratic indentation profile: force model for n=1 (SLS model)

To develop practical formulae for the force curves, we departed from the assumption that the indentation speed is constant in both load and unload portions of the force. Here we aim to generalize the discussion for nonlinear indentations. For a given indentation profile, the corresponding force is given by:

$$\bar{F}_L(t) = \int_0^t \bar{E}(t-t')\frac{d\bar{\delta}_L^\lambda(t')}{dt'}dt' \quad (t \le \tau_L) \tag{10}$$

$$\bar{F}_U(t) = \int_0^{\tau_L} \bar{E}(t-t')\frac{d\bar{\delta}_L^\lambda(t')}{dt'}dt' + \int_{\tau_L}^t \bar{E}(t-t')\frac{d\bar{\delta}_U^\lambda(t')}{dt'}dt' \quad (t \ge \tau_L) \tag{11}$$

Since $\bar{E}(t) = (1-\alpha) + \alpha e^{-t/\tau}$, the loading force becomes:

$$\bar{F}_L(t) = (1-\alpha)\bar{\delta}_L^\lambda(t) + \alpha \int_0^t e^{-(t-t')/\tau}\frac{d\bar{\delta}_L^\lambda(t')}{dt'}dt' \quad (t \le \tau_L) \tag{12}$$

$$\bar{F}_U(t) = (1-\alpha)\bar{\delta}_U^\lambda(t) + \alpha \int_0^{\tau_L} e^{-(t-t')/\tau}\frac{d\bar{\delta}_L^\lambda(t')}{dt'}dt' + \alpha \int_{\tau_L}^t e^{-(t-t')/\tau}\frac{d\bar{\delta}_U^\lambda(t')}{dt'}dt' \quad (t \ge \tau_L) \tag{13}$$

Analytical solutions for $\bar{F}_L(t)$ and $\bar{F}_U(t)$ strongly depends on the functional form of $\bar{\delta}(t)$. The indentation histories in AFM force curves are typically nonlinear for viscoelastic materials, they can be well represented by the following quadratic indentation ramp:

$$\bar{\delta}_L(t) = v_L t + \frac{b_L}{2}t^2 \quad (t \le \tau_L) \tag{14}$$

$$\bar{\delta}_U(t) = \bar{\delta}_L(\tau_L) - v_U(t-\tau_L) + \frac{b_U}{2}(t-\tau_L)^2 \quad (t \ge \tau_L). \tag{15}$$

Replacing this indentation profile in Eq. 12 results in complex integrals, for which analytical expressions can only be obtained for $\lambda = 2$. The load/unload force curves for conical indenter are:

$$\frac{\bar{F}_L(t)}{E_0} = (1-\alpha)\bar{\delta}_L^2(t) + 2\alpha\beta_L^2 \left[\left(\frac{12\gamma_L^2}{\beta_L^2} - \frac{6\gamma_L}{\beta_L} + 1\right)\left(e^{-t/\tau} + \frac{t}{\tau} - 1\right)\right] - \left[\left(\frac{12\gamma_L^2}{\beta_L^2} - \frac{6\gamma_L}{\beta_L}\right)\frac{1}{2}\frac{t^2}{\tau^2} - \frac{2\gamma_L^2}{\beta_L^2}\frac{t^3}{\tau^3}\right], \tag{16}$$

$$\frac{\bar{F}_U(t)}{E_0} = (1-\alpha)\bar{\delta}_U^2(t) + 2\alpha\beta_L^2 e^{-t/\tau}\left[\Gamma(2) - \Gamma\left(2, -\frac{1}{\beta_L}\right)\right] - \tag{17}$$

$$6\alpha\beta_L\gamma_L e^{-t/\tau}\left[\Gamma(3) - \Gamma\left(3, -\frac{1}{\beta_L}\right)\right] + 4\alpha\gamma_L^2 e^{-t/\tau}\left[\Gamma(4) - \Gamma\left(4, -\frac{1}{\beta_L}\right)\right] +$$

$$2\alpha\beta_U^2 e^{-(t-\tau_L)/\tau}\left[\Gamma(2) - \Gamma\left(2, -\frac{t-\tau_L}{\tau}\right) - \frac{\bar{\delta}_L(\tau_L)}{\beta_U}\left(1 - e^{(t-\tau_L)/\tau}\right)\right] +$$

$$6\alpha\beta_U\gamma_U e^{-(t-\tau_L)/\tau}\left[\Gamma(3) - \Gamma\left(3, -\frac{t-\tau_L}{\tau}\right)\right] +$$

$$4\alpha\gamma_U^2 e^{-(t-\tau_L)/\tau}\left[\Gamma(4) - \Gamma\left(4, -\frac{t-\tau_L}{\tau}\right) + \frac{\bar{\delta}_L(\tau_L)}{\gamma_U}\left(\Gamma(2) - \Gamma\left(2, -\frac{t-\tau_L}{\tau}\right)\right)\right].$$

where $\gamma_i = b_i\tau^2/2$ ($i = L, U$). We remark that it is more convenient to write the above expressions in time domain than in indentation domain. The linear indentation profile is a particular case of the quadratic indentation profile, and can obtained by making $\gamma_{L,U} = 0$ in the above equations.

## 3 Error analysis

Figure 2(a) compares linear and quadratic indentation profiles, where the amount of deviation from linear behavior can be controlled by the ratio $b_i\tau_L/(2v_i)$ $(i = L, U)$. The sign of $b_i$ can also be used to adjust experimental measurements. For small values of $|b_i\tau_L/2v_i| << 1$ one obtains a quasi-linear indentation profile.

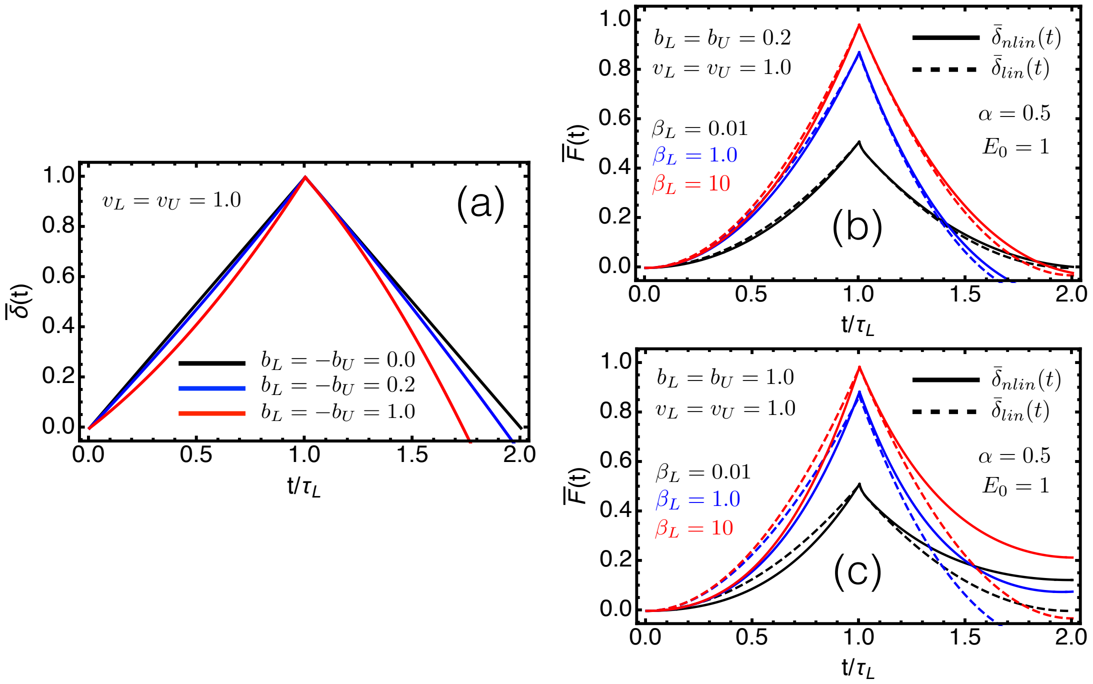


Figure 2: (a) Comparison of the linear and quadratic indentation profiles for different quadratic parameters. (b-c) Time domain forces curves calculated assuming linear (dashed lines) and quadratic (solid lines) indentation profiles. The forces curves were calculated for $\lambda = 2$ (conical indenter).

Figures 2(b)-(c) show the load/unload force curves in time domain for linear and quadratic indentations. For $b_i = 0.2$, the linear and quadratic models exhibit nearly identical force curves in both load and unload portions. The largest error occurs in the end of the unload portion, where functional method is not valid. For $b_i = 1.0$ there is a non-negligible difference between linear and quadratic models. The models only agree in three distinct parts: (i) in the begining and (ii) end of the load curve, and (iii) beginning of the unload curve. The difference between nonlinear and linear force curves $\Delta\bar{F}_L(t)/E_0$, where $\Delta\bar{F}_L(t) = \bar{F}_L^{nlin}(t) - \bar{F}_L^{lin}(t)$, for varying viscoelastic and nonlinear parameters is shown in Figure 3. The largest difference occurs for mid-range indentations between $\bar{\delta} = 0.4$ and $\bar{\delta} = 0.8$. The difference is proportional to both viscoelastic $\beta_L$ and nonlinear parameters $b_L\tau_L/2v_L$.

The indenter geometry has very little influence in the shape of $\Delta\bar{F}_L(t)/E_0$. The global error is shown in Figure 4 as function of $b_L/2v_L$ for representative combinations of the viscoelastic parameters $\alpha$ and $\beta_L$ spanning several order of magnitude. The global error is roughly linear up to $b_L\tau_L/2v_L = \pm 0.2$. Interestingly, the error is not symmetric with respect to the signal of the nonlinear parameter, such that it grows faster for negative values than for positives values of $b_L\tau_L/2v_L$. The error also grows with $\beta_L$ up to a maximum value that strongly depends on $b_L\tau_L/2v_L$, and it is inversely proportional to $\alpha$. But $\alpha$ and $\beta_L$ are connected: the error suffers larger variations with $\alpha$ for smaller values of $\beta_L$. For very large values of $\beta_L$, $\alpha$ has negligible influence. In conclusion, *the force curves obtained for the linear indentation profile can represent well force curves of nonlinear indentation profiles, as long as* $b_L\tau_L/2v_L$ *is small.*

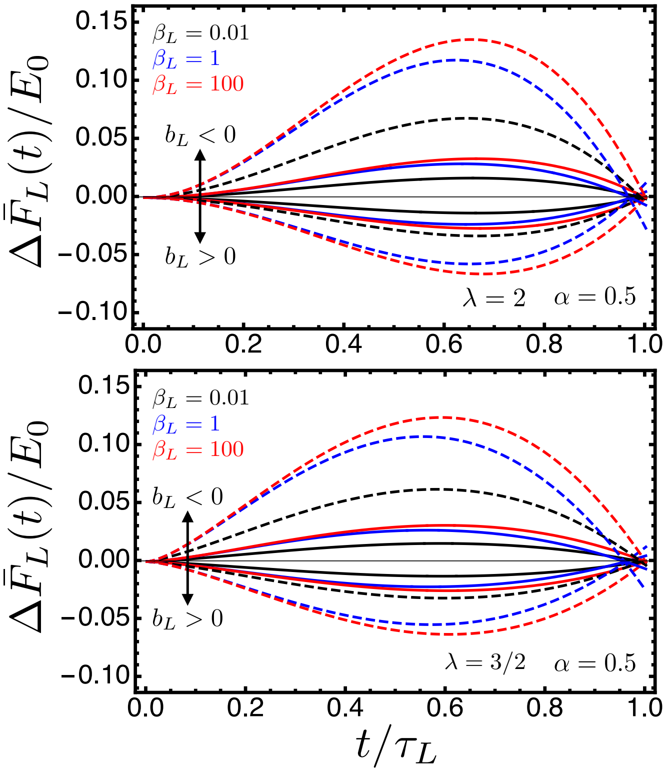


Figure 3: Difference between loading forces calculated with quadratic and linear indentation profiles ($\Delta\bar{F}_L(t) = \bar{F}_{L,nlin}(t) - \bar{F}_{L,nlin}(t)$) for several viscoelastic parameters spanning several orders of magnitude $\beta_L = 0.01$ (black), 1 (blue) and 100 (red). The nonlinear parameters are $b_L/2v_L = \pm 0.1$ (solid lines) and $\pm 0.3$ (dashed lines).

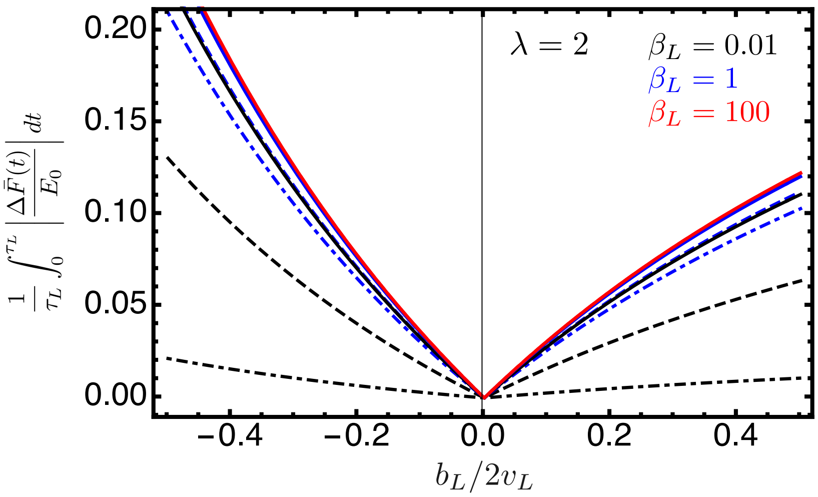


Figure 4: Global error during the loading curve for several viscoelastic parameters spanning several orders of magnitude $\beta_L = 0.01$ (black), 1 (blue) and 100 (red). $\alpha$ values are 0.1 (solid), 0.5 (dashed) and 0.95 (dot-dashed). This curve was computed for $\lambda = 2$, but nearly identical curves are obtained for $\lambda = 3/2$.

# 4 Computational FEM validation

We have calculated the time-dependent deformation of viscoelastic samples with FEM simulations. The adopted viscoelastic relaxation function in the simulations is the one of the SLS model (n=1). In short, our strategy to perform computational experiments of nanoindentation follows closely the one adopted in reference [Santos *et al.*, Soft Matter 8, 4441 (2012)]. Two types of axisymmetric indenters we used: conical (half-opening angles varying from $60^0$ to $80^0$) and spherical ($R = 1\ \mu m$). They were modeled as virtually undeformable in comparison to sample with elasticity modulus of $10^{13}$ Pa. The viscoelastic sample was modeled as thick enough to avoid finite thickness effects ($h = 3.5 \mu m$), and with instantaneous elasticity modulus of $E_0 = 10^6$ Pa. The values of the viscoelastic parameter $\alpha$ are chosen as $\alpha = 0.5, 0.95$.

To mimic the load phase of an AFM force curve, we have imposed as boundary condition $N_{tot} =$ 120 consecutive indentation steps at equally spaced time steps $\Delta t$ up to a maximum indentation of $\delta_{max} = 0.02 \mu m$, where $\delta_n = (n-1)\delta_{max}/(N_{tot} - 1)$ $(n = 1, ..., N_{tot})$. Then we compute the force $F_n$ necessary to achieve such indentations. The unload phase is equal to the load phase, but in reverse order. The total experiment time is $240\Delta t$, where $\Delta t$ is a scaling quantity. The investigated relaxation times spans in 4 orders of magnitude $\tau = 1.875\Delta t, 120\Delta t, 15360\Delta t$ such that $\beta_L = 0.0156, 1.0, 128$.

Figure 5 compares the force curves predicted by our analytical model and the ones obtained with FEM simulations for different viscoelastic parameters $\alpha$ and $\beta_L$ (we assumed $\beta_L = \beta_U$). We obtained a remarkable agreement between the analytical model and simulation for $\beta_L$ ratios spanning many orders of magnitude. Moreover, the analytical model is able to reproduce with great accuracy the unload curve in the limits $\beta_L \to 0$ and $\beta_L \to \infty$.

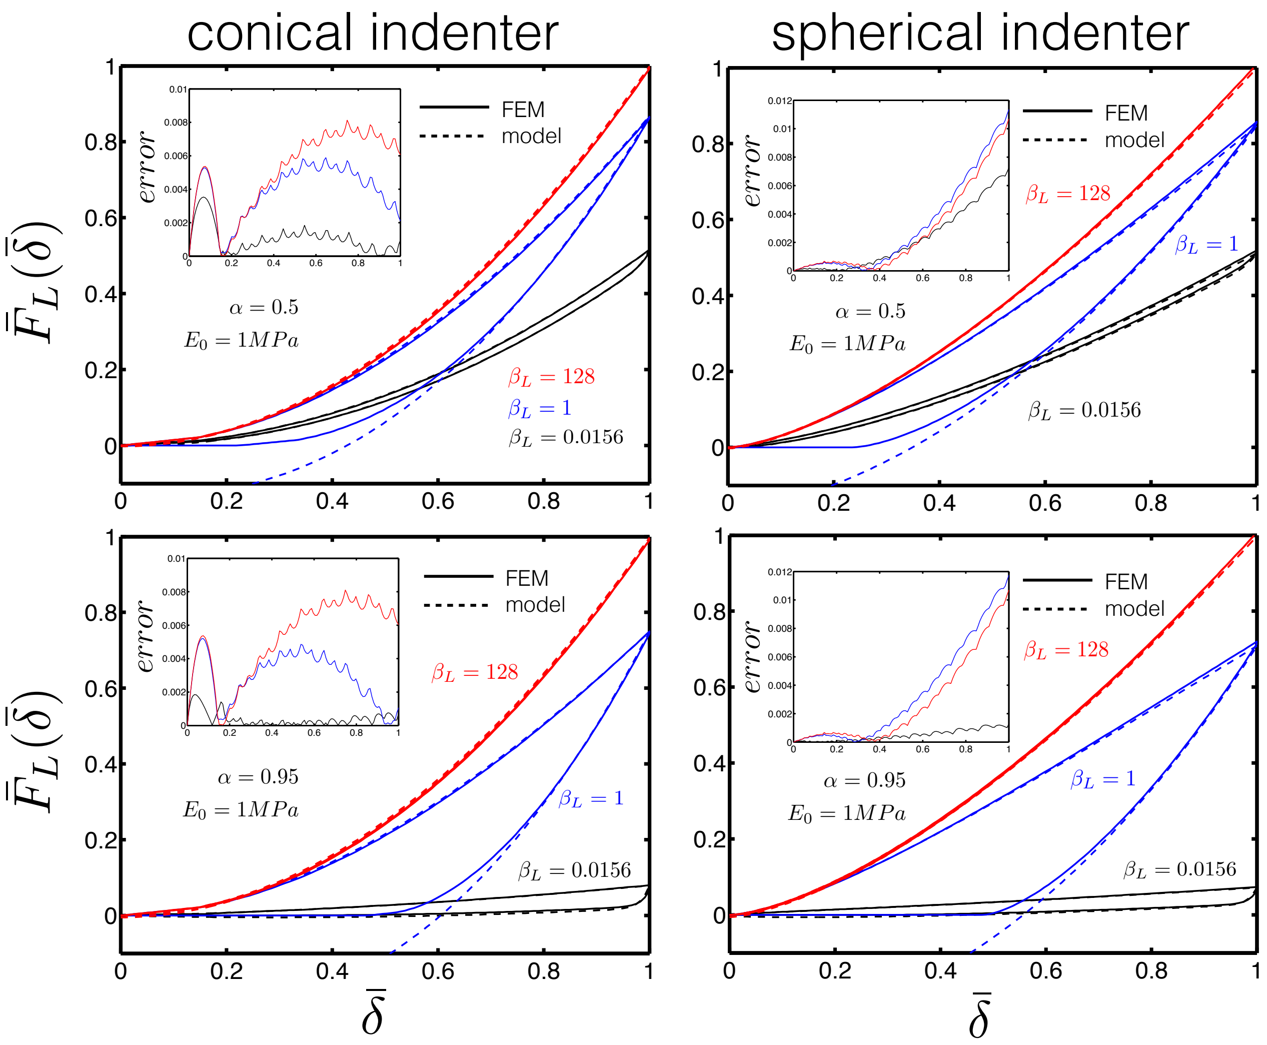


Figure 5: Comparison of force curves of conical ($\theta = 80^0$) and spherical ($R = 1\mu m$) indenters obtained with our analytical model and FEM simulations for different values of viscoelastic parameters $\alpha$ and $\beta_L$. We assumed $\beta_L = \beta_U$ in the FEM simulations. The error in the load curve computed as $|\bar{F}_L^{(model)}(\bar{\delta}) - \bar{F}_L^{(FEM)}(\bar{\delta})|$ is shown in the inset.

# 5 Indentation profiles of the polyacrylamide force curves

The normalized indentation histories of all force curves in this work are shown in Figure 6(a). All curves collapse in an universal quasi-linear quadratic indentation profile in both load/unload portions, and their nonlinear parameters are shown in Figure 6(b). For the load curves, this parameter remains nearly constant for all investigated frequencies, and grows with the bisacrylamide concentration. This trend is inverted for the unload curves. The largest measured values of $|b_i\tau_L/2v_i|$ are of the order of 0.2, indicating that the experimental force curves lie within the quasi-linear indentation regime.

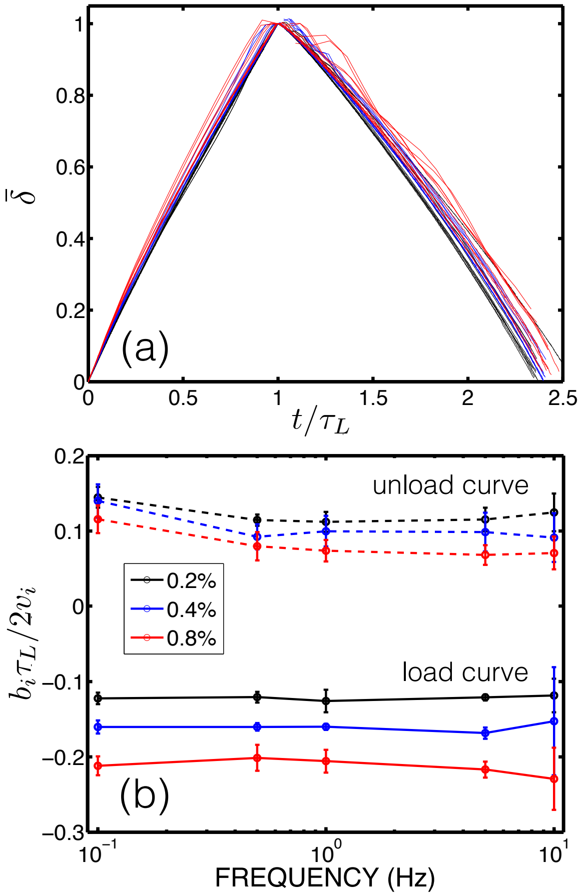


Figure 6: (a) Normalized indentation profiles of all force curves measured in this work. All curves collapse in a quasi-linear quadratic curve regardless frequency and bysacrilamide concentration. (b) Dependence of the mean values of the nonlinear parameters $b_i\tau_L/2v_i$ on the vertical scan frequency and bisacrylamide concentration.

# 6 Indentation profiles of the PnBMA force curves

Chyasnavichyus *et al.* investigated the viscoelastic properties of poly(n-butyl) methacrylate (PnBMA) polymers for different temperatures and loading rates. They constructed the PnBMA master curve using the frequency-temperature superposition principle from regular AFM force curves [Chyasnavichyus *et al.*, Langmuir **30**, 10566 (2014)]. Tthis polymer has a low glassy-transition temperature around 25$^o$C, such that one can easily access measure its viscoelastic behavior before and after the glassy-transition with frequencies between 0.1 Hz and 10 Hz. We took the liberty to construct the normalised indentation profiles of Chyasnavichyus' force curves (Figure 12 in reference Langmuir **30**, 10566 (2014)) to test the validity of our model concerning not only polymers with distinct viscoelastic behavior compared to polyacrylamide gels, but also to test our force model for spherical indenter geometry. Since Chyasnavichyus *et al.* modelled the PnBMA polymers with the SLS viscoelastic model, we fitted their data with fixed $n = 1$ only. Figure 7 shows that the assumption of linear indentation profiles works very well for PnBMA polymers. Chyasnavichyus *et al.* reported instantaneous and relaxed elasticity modulus of $E_0 = 958$ MPa and $E_\infty = 30$ MPa ($\alpha \approx 0.97$), which is compatible with all of our fitted values in Figure 7, except for the case T = $45^oC$ and $f_z = 10Hz$ in the middle of the rubbery-to-glassy transition. Our fitted relaxation times are also in agreement with the values determined by Chyasnavichyus *et al.* for temperatures above 40 $^oC$.

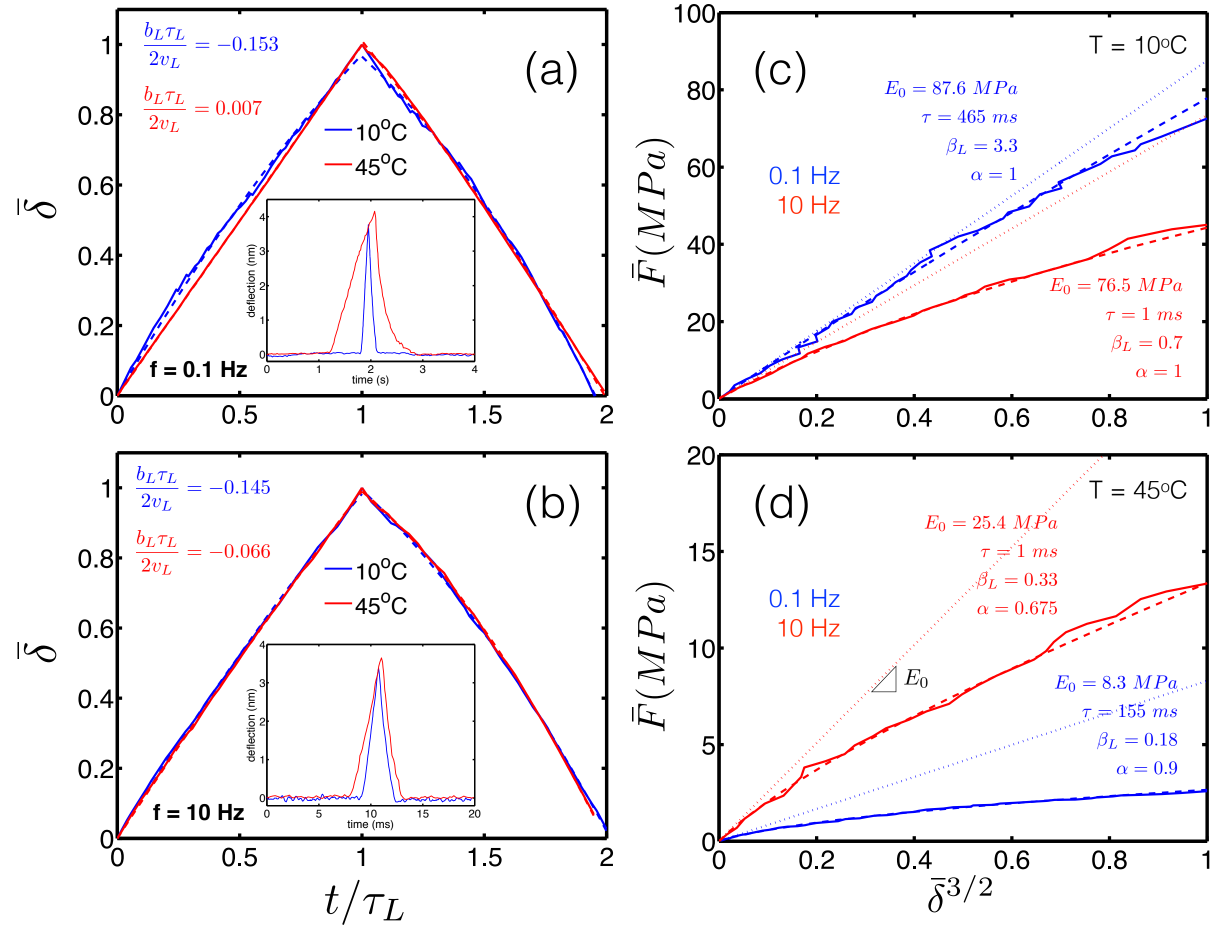


Figure 7: (a-b) Normalized indentation profiles constructed from the force curves measured in PnMBA with different vertical frequencies and temperatures by Chyasnavichyus *et al.*. The respective force curves in $d(t)$ form are shown in the inset graphs. According to the authors, the ramp size of all measurements were 150 nm, resulting in displacement speeds of 30 nm/s and 3000 nm/s for vertical frequencies of 0.1 Hz and 10 Hz, respectively. The average cantilever spring constant is 2 N/m. The average curvature radius of the AFM tips are $R = 30nm$. The dashed lines represent the fitting of the curves with a quadratic function whose nonlinear parameters for each case are shown in the graphs. (c-d) Normalised force curves of PnMBA. Solide lines are the constructed experimental curves, dashed lines represent the fitted force model for spherical indenters and linear indentation profile. The dotted lines represent the slope of the force curves near $\bar{\delta} = 0$.
